# Supplementary material for: HAPM -- Hardware Aware Pruning Method for CNN hardware accelerators in resource constrained devices
Source: arXiv:2408.14055 source file (2024-08-26)
Supplement: Supplementary file 1 [file 07-Appendix.tex]

\begin{figure*}
        \centering
        %\hspace*{-0.7in}
        
        \begin{tabular}{ccc}
        
        \subfloat[]{
            \begin{tikzpicture}[scale=0.4]
            \begin{axis}[xlabel=\spanish{Iteración}\english{Iteration},ylabel=\spanish{Exactitud}\english{Accuracy},y unit=\%,legend pos=south east]
                \addplot [color=red] table[x=Step,y=Value,col sep=comma] {data/01/train-tag-epoch_accuracy.csv};
                \addplot [color=blue] table[x=Step,y=Value,col sep=comma] {data/01/validation-tag-epoch_accuracy.csv};
                \addlegendentry{\spanish{Entrenamiento}\english{Training}}
                \addlegendentry{\spanish{Validación}\english{Validation}}
            \end{axis}
            \end{tikzpicture}
            %\label{<figure1>}
            } &
        
        \subfloat[]{
            \begin{tikzpicture}[scale=0.4]
            \begin{axis}[xlabel=\spanish{Iteración}\english{Iteration},ylabel=Función de pérdida,legend pos=north east]
                \addplot [color=red] table[x=Step,y=Value,col sep=comma] {data/01/train-tag-epoch_loss.csv};
                \addplot [color=blue] table[x=Step,y=Value,col sep=comma] {data/01/validation-tag-epoch_loss.csv};
                \addlegendentry{\spanish{Entrenamiento}\english{Training}}
                \addlegendentry{\spanish{Validación}\english{Validation}}
            \end{axis}
            \end{tikzpicture}
            %\label{<figure1>}
            } &
        
        \subfloat[]{
            \begin{tikzpicture}[scale=0.4]
            \begin{axis}[xlabel=\spanish{Iteración}\english{Iteration},ylabel=Factor de aprendizaje,legend pos=south east]
                \addplot [color=red] table[x=Step,y=Value,col sep=comma] {data/01/train-tag-epoch_lr.csv};
            \end{axis}
            \end{tikzpicture}
            \label{fig:version1_lr}
            } \\
        
        \end{tabular}
        \caption{\spanish{Curvas del entrenamiento de la primer versión del modelo}\english{Training curves of the first model}}
        \label{gra:primerversion_entrenamiento}
    \end{figure*}

\begin{figure*}
	\centering
	%\hspace*{-0.5in}
	
	\begin{tabular}{ccc}
		
		\subfloat[]{
			\begin{tikzpicture}[scale=0.4]
			\begin{axis}[xlabel=\spanish{Iteración}\english{Iteration},ylabel=Exactitud,y unit=\%,legend pos=south east]
			\addplot [color=red] table[x=Step,y=Value,col sep=comma] {data/02/train-tag-epoch_accuracy.csv};
			\addplot [color=blue] table[x=Step,y=Value,col sep=comma] {data/02/validation-tag-epoch_accuracy.csv};
			\addlegendentry{\spanish{Entrenamiento}\english{Training}}
			\addlegendentry{\spanish{Validación}\english{Validation}}
			\end{axis}
			\end{tikzpicture}
			%\label{<figure1>}
		} &
		
		\subfloat[]{
			\begin{tikzpicture}[scale=0.4]
			\begin{axis}[xlabel=\spanish{Iteración}\english{Iteration},ylabel=Función de pérdida,legend pos=north east]
			\addplot [color=red] table[x=Step,y=Value,col sep=comma] {data/02/train-tag-epoch_loss.csv};
			\addplot [color=blue] table[x=Step,y=Value,col sep=comma] {data/02/validation-tag-epoch_loss.csv};
			\addlegendentry{\spanish{Entrenamiento}\english{Training}}
			\addlegendentry{\spanish{Validación}\english{Validation}}
			\end{axis}
			\end{tikzpicture}
			%\label{<figure1>}
		} &
		
		\subfloat[]{
			\begin{tikzpicture}[scale=0.4]
			\begin{axis}[xlabel=\spanish{Iteración}\english{Iteration},ylabel=Factor de aprendizaje,legend pos=south east]
			\addplot [color=red] table[x=Step,y=Value,col sep=comma] {data/02/train-tag-epoch_lr.csv};
			\end{axis}
			\end{tikzpicture}
			%\label{<figure1>}
		} \\
		
	\end{tabular}
	\caption{\spanish{Curvas del entrenamiento de la segunda versión del modelo}\english{Training curves of the second model}}
	\label{gra:cuantizacion_entrenamiento}
\end{figure*}

\begin{figure*}
	\centering
	%\hspace*{-0.5in}
	\begin{tabular}{ccc}
		
		\subfloat[]{
			\begin{tikzpicture}[scale=0.4]
			\begin{axis}[xlabel=\spanish{Iteración}\english{Iteration},ylabel=Exactitud,y unit=\%,legend pos=south east]
			\addplot [color=red] table[x=Step,y=Value,col sep=comma] {data/03/train-tag-epoch_accuracy.csv};
			\addplot [color=blue] table[x=Step,y=Value,col sep=comma] {data/03/validation-tag-epoch_accuracy.csv};
			\addlegendentry{\spanish{Entrenamiento}\english{Training}}
			\addlegendentry{\spanish{Validación}\english{Validation}}
			\end{axis}
			\end{tikzpicture}
			%\label{<figure1>}
		} &
		
		\subfloat[]{
			\begin{tikzpicture}[scale=0.4]
			\begin{axis}[xlabel=\spanish{Iteración}\english{Iteration},ylabel=Función de pérdida,legend pos=north east]
			\addplot [color=red] table[x=Step,y=Value,col sep=comma] {data/03/train-tag-epoch_loss.csv};
			\addplot [color=blue] table[x=Step,y=Value,col sep=comma] {data/03/validation-tag-epoch_loss.csv};
			\addlegendentry{\spanish{Entrenamiento}\english{Training}}
			\addlegendentry{\spanish{Validación}\english{Validation}}
			\end{axis}
			\end{tikzpicture}
			%\label{<figure1>}
		} &
		
		\subfloat[]{
			\begin{tikzpicture}[scale=0.4]
			\begin{axis}[xlabel=\spanish{Iteración}\english{Iteration},ylabel=Factor de aprendizaje,legend pos=south east]
			\addplot [color=red] table[x=Step,y=Value,col sep=comma] {data/03/train-tag-epoch_lr.csv};
			\end{axis}
			\end{tikzpicture}
			%\label{<figure1>}
		} \\
		
	%	\subfloat[Capa 1]{
	%		\begin{tikzpicture}[scale=0.4]
	%		\begin{axis}[xlabel=Iteración,ylabel=Porcentaje en cero,y unit=\%,legend pos=south east]
	%		\addplot [color=red] table[x=Step,y=Value,col sep=comma] {data/03/prune_low_magnitude_conv2d_mask_0_sparsity.csv};
	%		%\addlegendentry{Entrenamiento}
	%		\end{axis}
	%		\end{tikzpicture}
	%		%\label{<figure1>}
	%	} &
	%	
	%	\subfloat[Capa 15]{
	%		\begin{tikzpicture}[scale=0.4]
	%		\begin{axis}[xlabel=Iteración,ylabel=Porcentaje en cero,y unit=\%,legend pos=north east]
	%		\addplot [color=red] table[x=Step,y=Value,col sep=comma] {data/03/prune_low_magnitude_conv2d_14_mask_0_sparsity.csv};
	%		%\addlegendentry{Entrenamiento}
	%		\end{axis}
	%		\end{tikzpicture}
	%		%\label{<figure1>}
	%	} &
	%	
	%	\subfloat[Capa 20]{
	%		\begin{tikzpicture}[scale=0.4]
	%		\begin{axis}[xlabel=Iteración,ylabel=Porcentaje en cero,y unit=\%,legend pos=south east]
	%		\addplot [color=red] table[x=Step,y=Value,col sep=comma] {data/03/prune_low_magnitude_conv2d_mask_0_sparsity.csv};
	%		\end{axis}
	%		\end{tikzpicture}
	%		%\label{<figure1>}
	%	} \\
		
	\end{tabular}
	\caption{\spanish{Curvas del entrenamiento de la tercer versión del modelo}\english{Training curves of the third model}}
	\label{gra:pruning_entrenamiento}
\end{figure*}

\begin{figure*}
	\centering
	%\hspace*{-0.5in}
	
	\begin{tabular}{ccc}
		
		\subfloat[]{
			\begin{tikzpicture}[scale=0.4]
			\begin{axis}[xlabel=\spanish{Iteración}\english{Iteration},ylabel=Exactitud,y unit=\%,legend pos=south east]
			\addplot [color=red] table[x=Step,y=Value,col sep=comma] {data/04/train-tag-epoch_accuracy.csv};
			\addplot [color=blue] table[x=Step,y=Value,col sep=comma] {data/04/validation-tag-epoch_accuracy.csv};
			\addlegendentry{\spanish{Entrenamiento}\english{Training}}
			\addlegendentry{\spanish{Validación}\english{Validation}}
			\end{axis}
			\end{tikzpicture}
			%\label{<figure1>}
		} &
		
		\subfloat[]{
			\begin{tikzpicture}[scale=0.4]
			\begin{axis}[xlabel=\spanish{Iteración}\english{Iteration},ylabel=Función de pérdida,legend pos=north east]
			\addplot [color=red] table[x=Step,y=Value,col sep=comma] {data/04/train-tag-epoch_loss.csv};
			\addplot [color=blue] table[x=Step,y=Value,col sep=comma] {data/04/validation-tag-epoch_loss.csv};
			\addlegendentry{\spanish{Entrenamiento}\english{Training}}
			\addlegendentry{\spanish{Validación}\english{Validation}}
			\end{axis}
			\end{tikzpicture}
			%\label{<figure1>}
		} &
		
		\subfloat[]{
			\begin{tikzpicture}[scale=0.4]
			\begin{axis}[xlabel=\spanish{Iteración}\english{Iteration},ylabel=Factor de aprendizaje,legend pos=south east]
			\addplot [color=red] table[x=Step,y=Value,col sep=comma] {data/04/train-tag-epoch_lr.csv};
			\end{axis}
			\end{tikzpicture}
			%\label{<figure1>}
		} \\
		
	\end{tabular}
	\caption{\spanish{Curvas del entrenamiento de la cuarta versión del modelo}\english{Training curves of the fourth model}}
	\label{gra:grouped_pruning_entrenamiento}
\end{figure*}
